# Supplementary material for: Hydra: Bidirectional State Space Models Through Generalized Matrix Mixers
Source: arXiv:2407.09941 source file (2024-07-13)
Supplement: Supplementary file 2 [file toeplitz.tex]

\makeatletter
\lst@UserCommand\lstrenewenvironment#1#2#{%
  \@ifundefined{#1}%
    {\PackageError{Listings}{Environment `#1' undefined}\@eha
     \@gobbletwo}\relax
  \expandafter\let\csname#1\endcsname\relax
  \expandafter\let\csname#1@\endcsname\relax
  \expandafter\let\csname end#1\endcsname\relax
  \let\lst@arg\@empty
  \lst@XConvert{#1}\@nil
  \expandafter\lstnewenvironment@\lst@arg{#1}{#2}}

% \lstrenewenvironment{python}[1][]{\lstset{style=mypython, #1}}{}
\lstrenewenvironment{python}[1][]{
    \lstset{style=mypython, basicstyle=\fontsize{7.5pt}{7.5pt}\ttfamily, #1}
}{}
% \lstrenewenvironment{python}[1][]{
%     \lstset{style=mypython, basicstyle=\footnotesize, #1}
% }{}
\makeatother

\begin{figure}[H]
    \centering
    \begin{python}[frame=top, frame=bottom]
class Toeplitz(nn.Module):
    def __init__(
        self,
        is_data_dependent,
        d_model,
        max_seq_len, # max_seq_len is necessary for Toeplitz.
        expand=2,
        headdim=128,
        device=None,
        dtype=None,
    ):
        factory_kwargs = {"device": device, "dtype": dtype}
        super().__init__()
        self.is_data_dependent = is_data_dependent
        self.d_model = d_model
        self.max_seq_len = max_seq_len
        self.expand = expand
        self.d_inner = self.expand * self.d_model
        self.headdim = headdim
        assert self.d_inner % self.headdim == 0
        self.nheads = self.d_inner // self.headdim

        self.kernel_size = 2 * self.max_seq_len - 1
        self.pad_size = self.max_seq_len - 1
        self.std_dev = 0.5 / np.sqrt(self.max_seq_len)

        if not self.is_data_dependent:
            self.conv_params = nn.Parameter(
                torch.empty(self.nheads, self.kernel_size, dtype=torch.float32, device=device)
            )
            nn.init.xavier_uniform_(self.conv_params)

    def forward(self, x, forward_conv=None, reverse_conv=None):
        """
        x: (batch, seqlen, nheads*headdim)
        forward_conv: (batch, seqlen, nheads)
        reverse_conv: (batch, seqlen, nheads)
        """
        residual = x
        x = rearrange(x, 'b l (n h) -> b h n l', n=self.nheads)

        # Pad the hidden states
        x = F.pad(x, (self.pad_size, 0))

        x_fft = torch.fft.fft(x.to(torch.float32), n=2*self.max_seq_len-1)
        if self.is_data_dependent:
            forward_conv = rearrange(forward_conv, 'b l n -> b n l')
            reverse_conv = rearrange(reverse_conv, 'b l n -> b n l')

            conv_params = torch.cat(
                [torch.flip(reverse_conv[:,:,1:], [-1]), forward_conv], dim=-1
            ).to(torch.float32) # FFT requires float32.
            fft_conv_params = torch.fft.fft(conv_params, n=self.kernel_size).unsqueeze(1)
        else:
            fft_conv_params = torch.fft.fft(self.conv_params, n=self.kernel_size)

        output = torch.fft.ifft(x_fft * fft_conv_params, n=self.kernel_size).real
        output = self.std_dev * output[:, :, :, :self.max_seq_len]
        output = rearrange(output, 'b h n l -> b l (n h)').to(residual.dtype) + residual

        return output
    \end{python}
    \vspace{-4mm}
    \caption{
        PyTorch code for the Toeplitz variants in~\cref{tab:abl_structures}.
    }
    \label{alg:toeplitz}
\end{figure}
