# Supplementary material for: Hydra: Bidirectional State Space Models Through Generalized Matrix Mixers
Source: arXiv:2407.09941 source file (2024-07-13)
Supplement: Supplementary file 3 [file vandermonde.tex]

\makeatletter
\lst@UserCommand\lstrenewenvironment#1#2#{%
  \@ifundefined{#1}%
    {\PackageError{Listings}{Environment `#1' undefined}\@eha
     \@gobbletwo}\relax
  \expandafter\let\csname#1\endcsname\relax
  \expandafter\let\csname#1@\endcsname\relax
  \expandafter\let\csname end#1\endcsname\relax
  \let\lst@arg\@empty
  \lst@XConvert{#1}\@nil
  \expandafter\lstnewenvironment@\lst@arg{#1}{#2}}

% \lstrenewenvironment{python}[1][]{\lstset{style=mypython, #1}}{}
\lstrenewenvironment{python}[1][]{
    \lstset{style=mypython, basicstyle=\fontsize{7.5pt}{7.5pt}\ttfamily, #1}
}{}
% \lstrenewenvironment{python}[1][]{
%     \lstset{style=mypython, basicstyle=\footnotesize, #1}
% }{}
\makeatother

\begin{figure}[H]
    \centering
    \begin{python}[frame=top, frame=bottom]
class Vandermonde(nn.Module):
    def __init__(
        self,
        is_data_dependent,
        d_model,
        qk_dim,
        is_dft=True,        # Used only when is_data_dependent is False.
        max_seq_len=None,   # max_seq_len is necessary for non-DFT data-independent version.
        expand=2,
        headdim=128,
        device=None,
        dtype=None,
    ):
        factory_kwargs = {"device": device, "dtype": dtype}
        super().__init__()
        self.is_data_dependent = is_data_dependent
        self.d_model = d_model
        self.qk_dim = qk_dim
        self.is_dft = is_dft
        self.max_seq_len = max_seq_len
        self.expand = expand
        self.d_inner = self.expand * self.d_model
        self.headdim = headdim
        assert self.d_inner % self.headdim == 0
        self.nheads = self.d_inner // self.headdim
        self.d_state = self.nheads * qk_dim

        if self.is_data_dependent:
            self.std_dev = 1 / np.sqrt(2 * self.max_seq_len * self.qk_dim)
            self.eps = 1e-3 # Constant to stabilize training.
        else:
            if self.is_dft:
                column_indices = torch.arange(self.max_seq_len)
                row_indices = torch.arange(self.max_seq_len).unsqueeze(1)
                dft_matrix = torch.cos(2 * torch.pi * row_indices * column_indices / self.max_seq_len).to(**factory_kwargs)
                self.register_buffer('dft_matrix', dft_matrix)
                self.std_dev = 1 / np.sqrt(self.max_seq_len)
            else:
                self.q_bias = nn.Parameter(torch.zeros(self.nheads, self.qk_dim, self.max_seq_len, **factory_kwargs))
                self.k_bias = nn.Parameter(torch.zeros(self.nheads, self.qk_dim, self.max_seq_len, **factory_kwargs))
                self.std_dev = 1 / np.sqrt(2 * self.max_seq_len * self.qk_dim)

    def forward(self, v, q=None, k=None):
        batch, seqlen, dim = v.shape
        residual = v
        v = rearrange(v, 'b l (n h) -> b l n h', n=self.nheads)
        if self.is_data_dependent:
            q = rearrange(q, 'b l (n d) -> b n d l', n=self.nheads)
            k = rearrange(k, 'b l (n d) -> b n d l', n=self.nheads)
            q_matrix = torch.cos(
                2 * torch.pi * self.eps * torch.einsum(
                    'b n d t, l -> b n d t l', q, torch.arange(seqlen, dtype=v.dtype).to(v.device)
                )
            )
            k_matrix = torch.cos(
                2 * torch.pi * self.eps * torch.einsum(
                    'b n d t, l -> b n d l t', k, torch.arange(seqlen, dtype=v.dtype).to(v.device)
                )
            )
            sym_vandermonde = (q_matrix - k_matrix).sum(dim=2)
            output = torch.einsum('b n t l, b l n h -> b t n h', sym_vandermonde, v)
        else:
            if self.is_dft:
                output = torch.einsum('b l n h, t l -> b t n h', v, self.dft_matrix)
            else:
                q, k = self.q_bias, self.k_bias
                q_matrix = torch.cos(
                    2 * torch.pi * torch.einsum(
                        'n d t, l -> n d t l', q, torch.arange(self.max_seq_len, dtype=v.dtype).to(v.device)
                    )
                )
                k_matrix = torch.cos(
                    2 * torch.pi * torch.einsum(
                        'n d t, l -> n d l t', k, torch.arange(self.max_seq_len, dtype=v.dtype).to(v.device)
                    )
                )
                sym_vandermonde = (q_matrix + k_matrix).sum(dim=1)
                output = torch.einsum('n t l, b t n h -> b t n h', sym_vandermonde, v)
        output = self.std_dev * output
        output = rearrange(output, 'b l n h -> b l (n h)') + residual
        return output
    \end{python}
    \vspace{-4mm}
    \caption{
        PyTorch code for the Vandermonde variants in~\cref{tab:abl_structures}.
    }
    \label{alg:vandermonde}
\end{figure}
