# Supplementary material for: Hydra: Bidirectional State Space Models Through Generalized Matrix Mixers
Source: arXiv:2407.09941 source file (2024-07-13)
Supplement: Supplementary file 4 [file broader_impact.tex]

\section{\textcolor{red}{Broader Impact}}
