# Supplementary material for: Hydra: Bidirectional State Space Models Through Generalized Matrix Mixers
Source: arXiv:2407.09941 source file (2024-07-13)
Supplement: Supplementary file 5 [file glue_std.tex]

\begin{table*}
\caption{
Evaluation on C4 dataset and GLUE Benchmark.
}
\vspace{-3mm}
\centering
\small
\resizebox{\linewidth}{!}
{ %< auto-adjusts font size to fill line
\begin{tabular}{lcccccccccccc} %@{}}
\toprule
\multirow{2}{*}{Method} & \multirow{2}{*}{\#Params} & \multicolumn{2}{c}{Pretrain} & \multicolumn{8}{c}{GLUE Tasks} & \multirow{2}[2]{*}{\begin{tabular}[c]{@{}c@{}}GLUE\\Avg\end{tabular}} \\ % \multirow{2}{*}{\shortstack{GLUE\\Avg}}
\cmidrule(lr){3-4}\cmidrule(lr){5-12}
                                        & & $\mathcal{L}_{ce}$  & Acc (\%) & MNLI & QNLI  & QQP   & RTE   & SST2  & MRPC  & COLA  & STS \\
\midrule
\multirow{2}{*}{Mamba} & \multirow{2}{*}{68M} & \multirow{2}{*}{3.45} & \multirow{2}{*}{39.5} \\
\\
\midrule
Add         & 70M \\
Mult        & 70M \\
Concat      & 69M \\
\rowcolor{lavender!30} Quasi    & 70M \\
\bottomrule
\end{tabular}
} %< \resizebox
\vspace{-4mm}
\label{tab:glue_std}
\end{table*}
