# Supplementary material for: Hydra: Bidirectional State Space Models Through Generalized Matrix Mixers
Source: arXiv:2407.09941 source file (2024-07-13)
Supplement: Supplementary file 6 [file attention.tex]

\makeatletter
\lst@UserCommand\lstrenewenvironment#1#2#{%
  \@ifundefined{#1}%
    {\PackageError{Listings}{Environment `#1' undefined}\@eha
     \@gobbletwo}\relax
  \expandafter\let\csname#1\endcsname\relax
  \expandafter\let\csname#1@\endcsname\relax
  \expandafter\let\csname end#1\endcsname\relax
  \let\lst@arg\@empty
  \lst@XConvert{#1}\@nil
  \expandafter\lstnewenvironment@\lst@arg{#1}{#2}}

% \lstrenewenvironment{python}[1][]{\lstset{style=mypython, #1}}{}
\lstrenewenvironment{python}[1][]{
    \lstset{style=mypython, basicstyle=\fontsize{7.5pt}{7.5pt}\ttfamily, #1}
}{}
% \lstrenewenvironment{python}[1][]{
%     \lstset{style=mypython, basicstyle=\footnotesize, #1}
% }{}
\makeatother

\begin{figure}[H]
    \centering
    \begin{python}[frame=top, frame=bottom]
class Attention(nn.Module):
    def __init__(
        self,
        is_data_dependent,
        d_model,
        qk_dim,
        max_seq_len=None,   # max_seq_len is necessary for data-independent version.
        expand=2,
        headdim=128,
        device=None,
        dtype=None,
    ):
        factory_kwargs = {"device": device, "dtype": dtype}
        super().__init__()
        self.is_data_dependent = is_data_dependent
        self.d_model = d_model
        self.qk_dim = qk_dim
        self.max_seq_len = max_seq_len
        self.expand = expand
        self.d_inner = self.expand * self.d_model
        self.headdim = headdim
        assert self.d_inner % self.headdim == 0
        self.nheads = self.d_inner // self.headdim
        self.d_state = self.nheads * qk_dim

        if not self.is_data_dependent:
            self.q_matrix = nn.Parameter(
                torch.empty(self.max_seq_len, self.nheads, self.qk_dim, **factory_kwargs))
            self.k_matrix = nn.Parameter(
                torch.empty(self.max_seq_len, self.nheads, self.qk_dim, **factory_kwargs))
            nn.init.xavier_normal_(self.q_matrix)
            nn.init.xavier_normal_(self.k_matrix)

    def forward(self, v, q=None, k=None):
        residual = v
        v = rearrange(v, 'b l (n h) -> b l n h', n=self.nheads)

        if self.is_data_dependent:
            q = rearrange(q, 'b l (n d) -> b l n d', n=self.nheads)
            k = rearrange(k, 'b l (n d) -> b l n d', n=self.nheads)
            qk = torch.einsum('b t n d, b l n d -> b n t l', q, k)
            attn_weights = torch.softmax(1 / np.sqrt(self.qk_dim) * qk, dim=-1)
            output = torch.einsum('b n t l, b l n h -> b t n h', attn_weights, v)
        else:
            qk = torch.einsum('n t d, n l d -> n t l', self.q_matrix, self.k_matrix)
            attn_weights = torch.softmax(1 / np.sqrt(self.qk_dim) * qk, dim=-1)
            output = torch.einsum('n t l, b l n h -> b t n h', attn_weights, v)

        output = rearrange(output, 'b l n h -> b l (n h)') + residual

        return output
    \end{python}
    \vspace{-4mm}
    \caption{
        PyTorch code for the Attention variants in~\cref{tab:abl_structures}.
    }
    \label{alg:attention}
\end{figure}
